# Supplementary material for: The exact two-spinon longitudinal dynamical structure factor of the anisotropic XXZ model
Source: arXiv:2005.10729 ancillary file (2020-05-21)
Supplement: Supplementary file 1 [file SupInfFinal.pdf]

# Supplemental Information: The exact two-spinon longitudinal dynamical structure factor of the anisotropic XXZ model

Isaac Pérez Castillo
*Department of Quantum Physics and Photonics, Institute of Physics,*
*UNAM, P.O. Box 20-364, 01000 Mexico City, Mexico and*
*London Mathematical Laboratory, 18 Margravine Gardens, London W6 8RH, United Kingdom*

In this Supplemental Information we provide detailed derivations for the two-spinon contribution to the longitudinal dynamical structure factor using quantum group approach.

## INTRODUCTION

In this Letter we have used the results of quantum group approach. Briefly speaking, this method works directly in the infinite lattice system and exploits a hidden symmetry: that of the universal enveloping algebra of $sl_2$, denoted as $U_q(sl_2)$, where $q$, usually called the deformation parameter, is related to the anisotropy parameter $\Delta$ by the formula

$$\Delta = \frac{q+q^{-1}}{2} \,. \tag{1}$$

Intuitively - and roughly - speaking, $U_q(sl_2)$ can be envisaged as a deformation of the commutation relations of the spin algebra $su(2)$. We will not discuss how this method is developed, taking instead a pragmatic view and simply enumerate what this method provides:

1. two vacuum states $|\text{vac}\rangle_{(i)}$ with $i=0,1$

2. eigenstates of the XXZ Hamiltonian, the so-called spinons, where and $m$-spinon state is denoted as $|\xi_m,\ldots\xi_1\rangle_{(i);\epsilon_m,\ldots,\epsilon_1}$. Here, the pair $(\xi_i,\epsilon_i)$ for each spinon $i=1,\ldots,m$ corresponds to the spectral parameters $\xi_i\in\mathbb{C}$ and the spinon's spin orientation $\epsilon_i\in -1,1$. This multi-spinon states have the property

$$\begin{aligned} H_{\text{XXZ}}\,|\xi_m,\ldots\xi_1\rangle_{(i);\epsilon_m,\ldots,\epsilon_1} &= \sum_i^m e(\xi_i)\,|\xi_m,\ldots\xi_1\rangle_{(i);\epsilon_m,\ldots,\epsilon_1} \\ T\,|\xi_m,\ldots\xi_1\rangle_{(i);\epsilon_m,\ldots,\epsilon_1} &= e^{i\sum_i^m p(\xi_i)}\,|\xi_m,\ldots\xi_1\rangle_{(1-i);\epsilon_m,\ldots,\epsilon_1} \end{aligned} \tag{2}$$

   where $T$ is the translation operator of one lattice site, and $p(\xi)$ and $e(\xi)$ are the momentum and energy of a spinon excitation.

3. The theory also provides a resolution of the identity in terms of spinons, viz.

$$\mathbb{1} = \sum_{m\geq 0}\sum_{\epsilon_1,\ldots,\epsilon_m}\frac{1}{m!}\sum_{p=0,\pi}\oint\prod_{i=1}^m\frac{d\xi_i^2}{2\pi i\xi_i^2}\,|\xi_m,\ldots\xi_1;p\rangle_{\epsilon_m,\ldots,\epsilon_1}\;{}_{\epsilon_1,\ldots,\epsilon_m}\langle\xi_1,\ldots,\xi_m;p|\;, \tag{3}$$

   which has been written in terms of translational invariant spinon states:

$$|\xi_m,\ldots,\xi_1;p\rangle_{\epsilon_m,\ldots,\epsilon_1} = \frac{1}{\sqrt{2}}\left[|\xi_m,\ldots\xi_1\rangle_{(0);\epsilon_m,\ldots,\epsilon_1} + e^{ip}\,|\xi_m,\ldots\xi_1\rangle_{(1);\epsilon_m,\ldots,\epsilon_1}\right]\,,\quad p=0,\pi \tag{4}$$

4. Finally, the quantum group approach also provides form factors for the components of the spin operator between vacuum states and the excited states, that is ${}_{(i)}\langle\text{vac}|\,\sigma_0^\alpha\,|\xi_m,\ldots\xi_1\rangle_{(i);\epsilon_m,\ldots,\epsilon_1}$, and also between vacuum states ${}_{(i)}\langle\text{vac}|\,\sigma_0^\alpha\,|\text{vac}\rangle_{(i)}$, for $\alpha\in\{x,y,z\}$

Notice that there is a complementary method to quantum group approach, which is algebraic Bethe ansatz. This method generates Bethe states for a given system size. Bethe states are labelled in terms of rapidities that obey Bethe equations. Algebraic Bethe ansatz does not provide simple formulas for form factors between two Bethe states so, instead, one is forced to numerically calcutate them. Luckily, the so-called Slavnov theorem helps to express form factors as determinants, which makes numerical evaluations much more efficient. The numerical approach to carry out this program is called ABACUS (Algebraic Bethe Ansatz-based Computation of Universal Structure factors) which was developed by one of the authors.

## LEHMANN REPRESENTATION OF THE DSF

We will start by writing the DSF in Lehmann representation. Let us denote the zero-temperature average as $\langle\cdots\rangle = \frac{1}{2}\sum_p \langle p|\cdots|p\rangle$. We write the following

$$S^{zz}(Q,\omega) = \frac{1}{4}\sum_{n=-\infty}^{\infty}\int_{-\infty}^{\infty} dt\, e^{i(\omega t - Qn)}\langle\sigma_n^z(t)\sigma_0^z(0)\rangle = \frac{1}{8}\sum_{n-\infty}^{\infty}\int_{-\infty}^{\infty} dt\, e^{i(\omega t-Qn)}\sum_{p,p'=0,\pi}\sum_{m\geq 0}\sum_{\epsilon_1,\dots,\epsilon_m}\frac{1}{m!}$$
$$\times\oint\prod_{i=1}^{m}\frac{d\xi_i^2}{2\pi i\xi_i^2}\langle p|\sigma_n^z(t)|\xi_m,\dots\xi_1;p'\rangle_{\epsilon_m,\dots,\epsilon_1\ \epsilon_1,\dots,\epsilon_m}\langle\xi_1,\dots,\xi_m;p'|\sigma_0^z|p\rangle \tag{5}$$

Now, since $\sigma_n^z(t) = T^{-n}e^{iHt}\sigma_0^z e^{-iHt}T^n$, with $T$ the translation operator for one lattice site, we have that:

$$\langle p|\sigma_n^z(t)|\xi_m,\dots\xi_1;p'\rangle_{\epsilon_m,\dots,\epsilon_1} = e^{-iE_m(\{\xi\})t+i[P_m(\{\xi\})+p'-p]n}\langle p|\sigma_0^z|\xi_m,\dots\xi_1;p'\rangle_{\epsilon_m,\dots,\epsilon_1} \tag{6}$$

Moreover:

$$\begin{aligned}\langle p|\sigma_0^z|\xi_m,\dots\xi_1;p'\rangle_{\epsilon_m,\dots,\epsilon_1} &= \frac{1}{2}\left[{}_{(0)}\langle\text{vac}| + e^{-ip}\,{}_{(1)}\langle\text{vac}|\right]\sigma_0^z\left[|\xi_m,\dots\xi_1\rangle_{(0);\epsilon_m,\dots,\epsilon_1} + e^{ip'}|\xi_m,\dots\xi_1\rangle_{(1);\epsilon_m,\dots,\epsilon_1}\right]\\ &= \frac{1}{2}\left[{}_{(0)}\langle\text{vac}|\sigma_0^z|\xi_m,\dots\xi_1\rangle_{(0);\epsilon_m,\dots,\epsilon_1} + e^{-i(p-p')}\,{}_{(1)}\langle\text{vac}|\sigma_0^z|\xi_m,\dots\xi_1\rangle_{(1);\epsilon_m,\dots,\epsilon_1}\right]\\ &= \frac{1}{2}\left[X^{(0)}_{\{\epsilon\}_m}(\{\xi\}_m) + e^{-i(p-p')}X^{(1)}_{\{\epsilon\}_m}(\{\xi\}_m)\right]\end{aligned} \tag{7}$$

where we have defined $X^{(i)}_{\{\epsilon\}_m}(\{\xi\}_m) \equiv {}_{(i)}\langle\text{vac}|\sigma_0^z|\xi_m,\dots\xi_1\rangle_{(i);\epsilon_m,\dots,\epsilon_1}$, as the form factor of the operator $\sigma_0^z$ connecting the vacuum state $i$ to its $m$-spinon excitation. Gathering results we write:

$$\begin{aligned}S^{zz}(Q,\omega) &= \frac{1}{32}\sum_{n=-\infty}^{\infty}\int_{-\infty}^{\infty} dt e^{i(\omega t-Qn)}\sum_{m\geq 0}\frac{1}{m!}\\ &\times\sum_{p,p'=0,\pi}\oint\prod_{i=1}^{m}\frac{d\xi_i^2}{2\pi i\xi_i^2}e^{-iE_m(\{\xi\})t+i[P_m(\{\xi\})+p'-p]n}\sum_{\{\epsilon\}_m}\left|X^{(0)}_{\{\epsilon\}_m}(\{\xi\}_m) + e^{-i(p-p')}X^{(1)}_{\{\epsilon\}_m}(\{\xi\}_m)\right|^2\\ &= \frac{1}{16}\sum_{m\geq 0}\frac{1}{m!}\oint\prod_{i=1}^{m}\frac{d\xi_i^2}{2\pi i\xi_i^2}\sum_{p=0,\pi}\\ &\times\sum_{n=-\infty}^{\infty}\int_{-\infty}^{\infty} dt e^{i(\omega-E_m(\{\xi\}))t-i(Q-P_m(\{\xi\})+p)n}\sum_{\{\epsilon\}_m}\left|X^{(0)}_{\{\epsilon\}_m}(\{\xi\}_m) + e^{ip}X^{(1)}_{\{\epsilon\}_m}(\{\xi\}_m)\right|^2\\ &= \frac{(2\pi)^2}{16}\sum_{m\geq 0}\frac{1}{m!}\oint\prod_{i=1}^{m}\frac{d\xi_i^2}{2\pi i\xi_i^2}\sum_{p=0,\pi}\delta[\omega-E_m(\{\xi\})]\delta_{(2\pi)}(Q-P_m(\{\xi\})+p)\sum_{\{\epsilon\}_m}\left|X^{(0)}_{\{\epsilon\}_m}(\{\xi\}_m) + e^{ip}X^{(1)}_{\{\epsilon\}_m}(\{\xi\}_m)\right|^2\end{aligned} \tag{8}$$

where in the last step we have used the Fourier representation for the Dirac delta

$$\sum_{n=-\infty}^{\infty} e^{-iAn} = 2\pi\delta_{(2\pi)}(A)\,, \qquad \int_{-\infty}^{\infty} dt e^{iAt} = 2\pi\delta(A)\,. \tag{9}$$

Therefore, the zero temperature DSF can be decomposed as a sum of $m$-spinon contributions

$$S^{zz}(Q,\omega) = \sum_{m\text{ even }\geq 0} S^{zz}_{(m)}(Q,\omega) \tag{10}$$

where $S^{zz}_{(m)}(Q,\omega)$ denotes the $m$-spinon contribution of the LDSF, and it has the following form:

$$\begin{aligned}S^{zz}_{(m)}(Q,\omega) &= \frac{\pi^2}{4}\frac{1}{m!}\oint\left[\prod_{i=1}^{m}\frac{d\xi_i^2}{2\pi i\xi_i^2}\right]\delta[\omega-E_m(\{\xi\})]\sum_{p=0,\pi}\delta_{(2\pi)}[Q+p-P_m(\{\xi\})]B^{(\sigma)}(\{\xi\}_m)\\ B^{(\sigma)}(\{\xi\}_m) &\equiv \sum_{\{\epsilon\}_m} B^{(\sigma)}_{\{\epsilon\}_m}(\{\xi\}_m)\,, \quad B^{(\sigma)}_{\{\epsilon\}_m}(\{\xi\}_m) \equiv \left|X^{(0)}_{\{\epsilon\}_m}(\{\xi\}_m) + \sigma X^{(1)}_{\{\epsilon\}_m}(\{\xi\}_m)\right|^2,\end{aligned} \tag{11}$$

with $\sigma = e^{ip}$. Following [20,22], it is fairly useful to work using the following parametrization of the spectral parameter

$$\xi = i e^{i\pi\beta/2K}\,, \quad -K \le \beta < K\,, \tag{12}$$

where $K \equiv K(k)$ is the complete elliptic integral of the first kind. The deformation parameter $q$ is chosen to be minus the elliptic nome $q_e$, $-q = q_e \equiv e^{-\frac{\pi K'}{K}}$, where $K' \equiv K(k')$, with $k' \equiv \sqrt{1-k^2}$ is the complementary elliptic modulus. Under this new parametrization, the spinon's energy and momentum take the following form:

$$e(\beta) = I \mathrm{dn}(\beta)\,, \quad p(\beta) = \mathrm{am}(\beta) + \frac{\pi}{2}\,, \quad I \equiv \frac{JK}{\pi}\sinh\left(\frac{\pi K'}{K}\right) \tag{13}$$

with $\mathrm{dn}(x) \equiv \mathrm{dn}(x,k)$ and $\mathrm{am}(x) \equiv \mathrm{am}(x,k)$ the usual Jacobi elliptic functions with elliptic modulus $k$. In this parametrization $S^{zz}_{(m)}(Q,\omega)$ takes the following form

$$S^{zz}_{(m)}(Q,\omega) = \frac{\pi^2}{4}\frac{1}{m!}\left(\prod_{i=1}^{m}\int_{-K}^{K}\frac{d\beta_i}{2K}\right)\delta[\omega - E_m(\{\beta\})]\sum_{p=0,\pi}\delta_{(2\pi)}[Q + p - P_m(\{\beta\})]B^{(\sigma)}(\{\beta\}_m)\,, \tag{14}$$

for all $m = 0, 2, 4, \ldots$. From Eq. (14) we see that we can use the two Dirac deltas to get rid of 2 out of the $m$ integrals over the $\beta$-parameters. In this Letter we have focused on the first two contributions corresponding $m = 0$ and $m = 2$. Let us discuss these two cases in detail.

## NO-SPINON CONTRIBUTION TO THE LDSF: STATIC CONTIRBUTION

The case $m = 0$ is static contribution and it does not involve any intregrals, viz.

$$S^{zz}_{(0)}(Q,\omega) = \frac{\pi^2}{4}\delta(\omega)\sum_{p=0,\pi}\delta_{(2\pi)}(Q+p)B^{(\sigma)}_{\mathrm{vac}}\,, \tag{15}$$

where we have used that $E_0(\{\beta\}) = 0$ and $P_0(\{\beta\}) = 0$ and denoted $B^{(\sigma)}(\{\beta\}_0) = B^{(\sigma)}_{\mathrm{vac}}$. Using the corresponding formulas from Jimbo and Miwa for these weights one obtains:

$$S^{zz}_{(0)}(Q,\omega) = \pi^2\delta(\omega)\delta_{(2\pi)}(Q)\prod_{n=1}^{\infty}\left(\frac{1-q^{2n}}{1+q^{2n}}\right)^4. \tag{16}$$

Notice that the total integrated intensity for $S^{zz}_0(Q,\omega)$, should give back squared staggered magnetization, that is

$$\int_0^{\infty}\frac{d\omega}{2\pi}\int_0^{2\pi}\frac{dQ}{2\pi}S^{zz}_{(0)}(Q,\omega) = \frac{1}{4}\prod_{n=1}^{\infty}\left(\frac{1-q^{2n}}{1+q^{2n}}\right)^4. \tag{17}$$

Finally, we point out that this expression can be written as the celebrated Baxter's formula as follows:

$$\begin{aligned}\frac{1}{4}\prod_{n=1}^{\infty}\left(\frac{1-q^{2n}}{1+q^{2n}}\right)^4 &= \frac{1}{4}\prod_{n=1}^{\infty}\left(\frac{q^{-n}-q^{n}}{q^{-n}+q^{n}}\right)^4 = \frac{1}{4}\prod_{n=1}^{\infty}\left[\tanh\left(n\frac{\pi K'}{K}\right)\right]^4\\ &= \frac{1}{4}\prod_{n=1}^{\infty}\tanh^4\left[n\,\mathrm{acosh}(\Delta)\right]\end{aligned} \tag{18}$$

where we have used that $q = q_e = e^{-\frac{\pi K'}{K}}$ and $\cos(\frac{\pi K'}{K}) = \Delta$.

## TWO-SPINON CONTRIBUTION TO THE LDSF

Particularising this expression for $m = 2$ we obtain

$$S^{zz}_{(2)}(Q,\omega) = \frac{\pi^2}{8}\left(\frac{1}{2K}\right)^2\int_{-K}^{K}\int_{-K}^{K}d\beta_1 d\beta_2\,\delta[\omega - E_2(\beta_1,\beta_2)]\sum_{p=0,\pi}\delta_{(2\pi)}[Q+p-P_2(\beta_1,\beta_2)]B^{(\sigma)}(\beta_1,\beta_2)\,. \tag{19}$$

According to the expression (19), to find an exact expression of $S^{zz}_{(2)}(Q,\omega)$ we must: i) resolve the two-spinon energy-momentum dispersion relation in terms of the $\beta$-parameters; ii) use this relationship to evaluate the weights $B^{(\sigma)}(\beta_1,\beta_2)$ that contain the two-spinon form factors of the operator $\sigma^z$. Before discussing these two steps, a few words are in order. The first step was correctly done for the first time in [20] and, for brevity we will only recall the main formulas. The second step, evaluating $B^{(\sigma)}(\beta_1,\beta_2)$, has a serious problem: the expression of the form factor ${}_{(i)}\langle\mathrm{vac}|\,\sigma^z_0\,|\xi_2,\xi_1\rangle_{\epsilon_2,\epsilon_1;(i)}$ given by the quantum group approach [11] involve two innocent-looking coupled contour integrals, which must be first evaluated to have a compact expression of the said form factor. We will point out what is the main mathematical obstacle when evaluating these contour integrals and we will briefly discuss and strategy of how to tackle this type of problem. We will use, however, a compact expression for this weight which was recently found by other means.

**About the form factor ${}_{(i)}\langle\mathrm{vac}|\,\sigma^z_0\,|\xi_2,\xi_1\rangle_{\epsilon_2,\epsilon_1;(i)}$**

Jimbo and Miwa quantum group results [11] give expressions for ${}_{(i)}\langle\mathrm{vac}|\sigma^z_0|\xi_2,\xi_1\rangle_{\epsilon_2,\epsilon_1;(i)}$ that thus far have avoided an evaluation. Although we have developed a method to evaluate such daunting contour integral, the resulting expression is horribly complicated [16]. In the main text we have instead used the results found in [17,18,19] which provides a compact expression directly for the $B$-weights. Before doing so, we think to be worth to briefly discussing the underlying mathematical problem when evaluating this form factor directly from the expressions provided in [11]. This form factor is given by the following formula. Let us first note that from a all possible spin orientations only those $(\epsilon_1,\epsilon_2)=\{(+,-),(-,+)\}$ have a non-zero form factor. If we denote with $\ell$ the position of the plus sign in the previous sets the we can write the corresponding form factor $X^{(i)}_\ell(\xi_2,\xi_1)$ as follows

$$\begin{aligned} X^{(i)}_\ell(\xi_2,\xi_1) &= (-q)^{-i}(1-q^{-2})(q^2;q^4)^3_\infty(q^4;q^4)^5_\infty\rho^2\frac{\gamma(\xi_2^2/\xi_1^2)}{\prod_{k=1,2}\Theta_{q^4}(q\xi_k^2)}\prod_{k=1,2}\xi_k^{k-(1+\epsilon_k)/2-i} \\ &\times\oint_{\widetilde{C}}\frac{dv}{2\pi iv}\prod_{k<\ell}(qv^{-1}-q^{-1}u_k^{-1})\prod_{k>\ell}(v^{-1}-u_k^{-1})\frac{(-q^{-1}v;q^2)_\infty(-q^3/v;q^2)_\infty}{\prod_{k=1,2}(u_k/v;q^4)_\infty(q^{-2}v/u_k;q^4)_\infty} \\ &\times(-v)^i\,G^z_i(v,u)\,, \end{aligned} \tag{20}$$

with

$$\begin{aligned} G^z_i(v,\{u\}) &= \oint_{C^++C^-}\frac{dw}{2\pi iw}\frac{w^{1-i}}{(w;q^2)_\infty(q^2/w;q^2)_\infty}\frac{\prod_{k=1,2}(-qu_k/w;q^4)_\infty(-q^3w/u_k;q^4)_\infty}{(-q^{-1}v/w;q^2)_\infty(-q^3w/v;q^2)_\infty} \\ &\times\Theta_{q^8}\left(-q^{4i}\frac{v^2}{w^2\prod_{k=1,2}u_k}\right)\,. \end{aligned} \tag{21}$$

Here the contour $\widetilde{C}$ is such that $q^{4n}u_k$ $(n\ge 0)$ are inside the contour and $C^\pm$ are such that $q^{2\ell+1\pm1}$ $(\ell\ge0)$ and $-q^{1+2\ell}v$ $(\ell\ge0)$ are inside the contour. Also the $\Theta_q$-symbol is defined as

$$\Theta_q(w)\equiv(w;q)_\infty(qw^{-1};q)_\infty(q;q)_\infty\,,\quad (w;q)_\infty\equiv\prod_{n=0}^{\infty}(1-wq^n) \tag{22}$$

We also introduce for later use

$$\begin{aligned} (w;q,p)_\infty &\equiv \prod_{n,m=0}^{\infty}(1-wq^np^m)\,, \\ \gamma_\sigma(w) &\equiv \frac{((-q)^{1+\sigma}q^4w;q^4,q^4)_\infty((-q)^{1+\sigma}w^{-1};q^4,q^4)_\infty}{((-q)^{3+\sigma}q^4w;q^4,q^4)_\infty((-q)^{3+\sigma}w^{-1};q^4,q^4)_\infty} \end{aligned} \tag{23}$$

so that our usual $\gamma(w)\equiv\gamma_-(w)$ while $\rho^2\equiv\gamma_+(q^{-2})$. Obviously, one would be tempted to evaluate the contour integrals appearing in the expression (20) by applying the residues theorem. There is a problem though: the integrand regarding the integration variable $w$ can we written in terms of $\Theta_q$-functions which enjoy the so-called quasi-periodicity property. This can be used to show that the corresponding contours can be deformed by adding and subtracting subsets of poles while keeping the value of the integral unchanged: that is, the overall contribution coming from the residues of various simple poles cancel each other. This is somewhat an odd property of the integrand and, since we do not expect this form factor to be zero, this forcibly implies that

the whole contribution to the integral comes from an essentially singularity at $w = 0$ (and perhaps a few ones that appear when contracting the contour to a radius infinitesimally small around zero). Since the integrand is given as ratios of infinite products, evaluating this essentially singularity directly is a hopeless task. However, if we could expand the integrand as a Laurent series within a band not containing poles, then we can integrate the series term by term and the problem would be resolved. We will illustrate this with a very simple example that has precisely this problem and can be applied to any form factor for the operator $\sigma^z$.

Let us pinpoint the issue of the contour integral by means of the following example. Consider the integrand:

$$\mathcal{I}(w) = \frac{[\Theta_{q^4}(-q/w)]^2}{\Theta_{q^2}(-1/w)}\,, \tag{24}$$

which has poles at $w = -q^{2n}$ and $w = -q^{-2-2n}$ with $0 < q < 1$, and let $C$ be a close contour which contains only the first set of poles. Notice that, under the transformation $w = \hat{w}q^{-4}$, the integrand has the following property, due to the quasi-periodicity property of the $\Theta_q$ function:

$$\mathcal{I}(\hat{w}q^{-4}) = \mathcal{I}(\hat{w})\,, \tag{25}$$

This automatically implesi that the contour intetgral transforms as follows:

$$\mathcal{I} = \oint_C \frac{dw}{2\pi i w}\frac{[\Theta_{q^4}(-q/w)]^2}{\Theta_{q^2}(-1/w)} = \oint_{\widehat{C}} \frac{d\hat{w}}{2\pi i\hat{w}}\frac{[\Theta_{q^4}(-q/\hat{w})]^2}{\Theta_{q^2}(-1/\hat{w})}\,, \tag{26}$$

where the new contour $\widehat{C}$ is such that the poles $\hat{w} = -q^{4+2n}$ $(n \geq 0)$ are inside the closed contour and $w = q^{2-2n}$ $(n \geq 0)$ are outside. Thus the overall contribution coming from the residues of the poles at $w = 1$ and $w = q^2$ must cancel each other, as this is the only difference between the two contours (of course one can indeed check this with a simple derivation). Clearly this transformation can be repeated to bring the contour just to be infinitesimally around $w = 0$. Since we know that numerically the integral is different from zero, this implies that there is something else going on at $w = 0$ other than simple poles. Before tackling this, we leave as an exercise to indeed check that, applying the theorem of residues to only the simple poles is hopeless, since one gets:

$$\begin{aligned}\mathcal{I} &= \frac{[\Theta_{q^4}(q)]^2}{(q^2;q^2)^3_\infty}\sum_{m=0}^{\infty}\left[q^{2m(2m+1)}q^{-2m(2m+1)} - q^{(2m+1)(2m+2)}q^{-(2m+1)(2m+2)}\right] \\ &\stackrel{?}{=} 0\end{aligned} \tag{27}$$

So we conclude that to successfully evaluate the contour integral in this case, everything boils down to evaluate the residue coming from an essential singularity around zero. However, evaluating the residues coming from essentially singularities is not always an easy task. To tackle this problem, let us first recall the following Ramanujan's ${}_1\Psi_1$ summation formula

$$\frac{(\alpha t;p)_\infty(p/\alpha t;p)_\infty(\beta/\alpha;p)_\infty(p;p)_\infty}{(t;p)_\infty(\beta/\alpha t;p)_\infty(\beta;p)_\infty(p/\alpha;p)_\infty} = \sum_{n=-\infty}^{\infty}\frac{(\alpha;p)_n}{(\beta;p)_n}t^n \tag{28}$$

for $|\beta/\alpha| < |t| < 1$ and with

$$(a;q)_n = \frac{(a;q)_\infty}{(aq^n;q)_\infty} = \prod_{k=0}^{n-1}(1-aq^k) \tag{29}$$

Using Eq. 28 allows us to write the following two Laurent expansions:

$$\frac{\Theta_{q^4}(-q^3w)}{\Theta_{q^4}(-q^2w)} = \frac{(q^5;q^4)_\infty(q^3;q^4)_\infty}{(q^4;q^4)^2_\infty}\sum_{n=-\infty}^{\infty}\frac{(q,q^4)_n}{(q^5,q^4)_n}(-1)^n q^{2n}w^n\,, \qquad q^2 < |w| < q^{-2}\,, \tag{30}$$

and

$$\frac{\Theta_{q^4}(-q^3w)}{\Theta_{q^4}(-q^4w)} = \frac{(q^3;q^4)_\infty(q^5;q^4)_\infty}{(q^4;q^4)^2}\sum_{n=-\infty}^{\infty}\frac{(q^{-1},q^4)_n}{(q^3,q^4)_n}(-1)^n q^{4n}w^n\,, \qquad 1 < |w| < q^{-4}\,. \tag{31}$$

Note that the two annulus of convergence have the common annulus $1 < |w| < q^{-2}$. Luckily this annulus is such that can contain precisely the close contour involved in the contour integral. As the two series are absolute convergent inside the annulus we can proceed to integrate term by term. Indeed, we can do now the following steps:

$$\begin{aligned}
\mathcal{I} &= \oint_C \frac{dw}{2\pi i w} \frac{[\Theta_{q^4}(-q/w)]^2}{\Theta_{q^2}(-1/w)} = \frac{(q^2;q^2)_\infty}{(q^4;q^4)^2_\infty} \oint_C \frac{dw}{2\pi i w} \frac{\Theta_{q^4}(-q^3 w)}{\Theta_{q^4}(-q^2 w)} \frac{\Theta_{q^4}(-q^3 w)}{\Theta_{q^4}(-q^4 w)} \\
&= \frac{(q^2;q^2)_\infty}{(q^4;q^4)^2_\infty} \left[ \frac{(q^5;q^4)_\infty (q^3;q^4)_\infty}{(q^4;q^4)^2_\infty} \right]^2 \sum_{n,m=-\infty}^{\infty} \frac{(q,q^4)_n}{(q^5,q^4)_n} \frac{(q^{-1},q^4)_m}{(q^3,q^4)_m} (-1)^{n+m} q^{2n+4m} \oint_C \frac{dw}{2\pi i} w^{n+m-1} \\
&= \frac{(q^2;q^2)_\infty}{(q^4;q^4)^2_\infty} \left[ \frac{(q^5;q^4)_\infty (q^3;q^4)_\infty}{(q^4;q^4)^2_\infty} \right]^2 \sum_{n,m=-\infty}^{\infty} \frac{(q,q^4)_n}{(q^5,q^4)_n} \frac{(q^{-1},q^4)_m}{(q^3,q^4)_m} (-1)^{n+m} q^{2n+4m} \delta_{m,-n} \\
&= \frac{(q^2;q^2)_\infty}{(q^4;q^4)^2_\infty} \left[ \frac{(q^5;q^4)_\infty (q^3;q^4)_\infty}{(q^4;q^4)^2_\infty} \right]^2 \sum_{n=-\infty}^{\infty} \frac{(q,q^4)_n}{(q^5,q^4)_n} \frac{(q^{-1},q^4)_{-n}}{(q^3,q^4)_{-n}} q^{-2n} .
\end{aligned} \tag{32}$$

Finally using the property:

$$(a,q)_{-n} = \frac{1}{(aq^{-n};q)_n} = \frac{(-q/a)^n q^{n(n-1)/2}}{(q/a;q)_n} , \tag{33}$$

we end up wit the correct formula of the contour integral of our illustrative example (Nb. One can check this formula is indeed correct by comparing it with results from numerical integration)

$$\mathcal{I} = \frac{1}{(q^2;q^2)_\infty} \left[ \frac{(q^5;q^4)_\infty (q^3;q^4)_\infty}{(q^4;q^4)_\infty} \right]^2 \sum_{n=-\infty}^{\infty} \frac{(q,q^4)^2_n}{(q^5,q^4)^2_n} q^{2n} . \tag{34}$$

### Expression for the $B^{(\sigma)}(\beta_1, \beta_2)$ weights for the two-spinon contribution

As we have previously emphasized we have now a way to evaluate multi-spinon form factor for the operator $\sigma^z$. This can be applied to the particular problem we are interested in, however, luckily for us, a compact expression has been already found [17,18,19]. What we are left to do is the rather tedious task of expressing it in term of elliptic functions and used the expression of the two-spinon energy-momentum dispersion relation.

As the author in [19] use a different notation and parametrization, let us thread with care to find the weights $B^{(\sigma)}(\beta_1, \beta_2)$. We first recall from[19], that the zero-spinon and two-spinon contribution to the longitudinal correlation function is

$$\left\langle \sigma_1^z \sigma_{m+1}^z(t) \right\rangle_2 = \frac{(q^2;q^2)^4}{(-q^2;q^2)^4} (-1)^m + \frac{1}{2} I_2(m,t) , \tag{35}$$

with

$$I_2(m,t) = \left[ \prod_{j=1}^{2} \int_{-\frac{\pi}{2}}^{\frac{\pi}{2}} \frac{d\nu_j}{2\pi} e^{i[p(\nu_j)m - \epsilon(\nu_j)t]} \right] f(\nu_1,\nu_2) . \tag{36}$$

Here the function $f(\nu_1, \nu_2)$ is defined as

$$f(\nu_1,\nu_2) = A(\nu_1,\nu_2)(-1)^m + A(\nu_1+\pi,\nu_2) \tag{37}$$

with

$$\begin{aligned}
A(\nu_1,\nu_2) = &\frac{32q(q^2;q^2)^2 \cos^2((p(\nu_1)+p(\nu_2))/2) \sin^2(\nu_{12}) \theta_4^2(\nu_{12}/2,q)}{\sin((\nu_{12}+i\gamma)/2)\sin((\nu_{12}-i\gamma)/2)} \\
&\times \prod_{\sigma=\pm} \frac{(q^4;q^4,q^4)^2 (q^4 e^{2i\sigma\nu_{12}};q^4,q^4)^2 (q^4 e^{2i\sigma\nu_{12}};q^4)}{(q^2;q^4,q^4)^2 (q^2 e^{2i\sigma\nu_{12}};q^4,q^4)^2 (q^2 e^{2i\sigma\nu_{12}};q^4)} ,
\end{aligned} \tag{38}$$

and $\nu_{12} = \nu_1 - \nu_2$. This $A$ coefficients are precisely our weights.

Seeking for a more compact expression for $A(\nu_1,\nu_2)$, we will rewrite it in terms of of Jacobi elliptic functions. Let us start by noticing that, within their definitions, we take the deformation parameter $q$ to be precisely the elliptic nome, that is $q = q_e$. Next, let us recall the following properties of the Jacobi theta functions:

$$\begin{aligned}
\theta_4(q) &= (q^2;q^2)(q;q^2)^2 = \sqrt{\frac{2k'K}{\pi}}\,, \\
\theta_2(q) &= 2q^{1/4}(-q^2;q^2)^2(q^2;q^2) = \sqrt{\frac{2kK}{\pi}}\,, \\
\theta_3(q) &= (q^2;q^2)(-q;q^2)^2 = \sqrt{\frac{2K}{\pi}}\,.
\end{aligned} \tag{39}$$

From the function $\gamma_\sigma(w)$, we have that

$$\begin{aligned}
\gamma_-(q^{-2}) &= \frac{(q^2;q^4,q^4)^2}{(q^4;q^4,q^4)^2}\,, \quad \gamma_+(q^{-2}) = \frac{(q^4;q^4,q^4)^2}{(q^6;q^4,q^4)^2}\,, \\
\gamma_-(w) &= \frac{(wq^4;q^4,q^4)(w^{-1};q^4,q^4)}{(wq^6;q^4,q^4)(w^{-1}q^2;q^4,q^4)}\,.
\end{aligned} \tag{40}$$

The following derivation consists in rewriting the various terms appearing in the expression of $A(\nu_1,\nu_2)$. It is not difficult to convince one-self that:

$$\begin{aligned}
(q^2e^{2i\nu_{12}};q^4)(q^2e^{-2i\nu_{12}};q^4) &= \frac{\theta_4(q^2)}{\theta_3(q)\theta_4(q)}\frac{1}{(q^4;q^4)}\theta_4(e^{i\nu_{12}/2},q)\theta_3(e^{i\nu_{12}/2},q)\,, \\
(q^4e^{2i\nu_{12}};q^4)(q^4e^{-2i\sigma\nu_{12}};q^4) &= \frac{\theta_4(q^2)}{\theta_3(q)\theta_4(q)}\frac{1}{2\sin(\nu_{12})(q^4;q^4)}\frac{\theta_1(e^{i\nu_{12}/2},q)\theta_2(e^{i\nu_{12}/2},q)}{\sqrt{q}}\,.
\end{aligned} \tag{41}$$

Thus far we have the following intermediate expression for $A(\nu_1,\nu_2)$:

$$\begin{aligned}
A(\nu_1,\nu_2) = {}& \frac{32q(q^2;q^2)^2\cos^2((p(\nu_1)+p(\nu_2))/2)\sin^2(\nu_{12})\vartheta_4^2(\nu_{12}/2,q)}{\sin((\nu_{12}+i\gamma)/2)\sin((\nu_{12}-i\gamma)/2)} \\
&\times \prod_{\sigma=\pm}\frac{(q^4;q^4,q^4)^2(q^4e^{2i\sigma\nu_{12}};q^4,q^4)^2}{(q^2;q^4,q^4)^2(q^2e^{2i\sigma\nu_{12}};q^4,q^4)^2} \\
&\times \frac{1}{2\sqrt{q}\sin(\nu_{12})}\frac{\theta_1(e^{i\nu_{12}/2},q)\theta_2(e^{i\nu_{12}/2},q)}{\theta_4(e^{i\nu_{12}/2},q)\theta_3(e^{i\nu_{12}/2},q)}
\end{aligned} \tag{42}$$

To have a compact expression, similar to the transverse case, we further notice that:

$$\frac{(q^4;q^4,q^4)^2}{(q^2;q^4,q^4)^2} = \frac{(q^4;q^4,q^4)^2}{(q^2;q^4)^2(q^6;q^4,q^4)^2} = \frac{\rho^2}{(q^2;q^4)^2}\,, \tag{43}$$

where we have defined $\rho^2 \equiv \gamma_+(q^{-2})$, and

$$\prod_{\sigma=\pm}\frac{(q^4e^{2i\sigma\nu_{12}};q^4,q^4)^2}{(q^2e^{2i\sigma\nu_{12}};q^4,q^4)^2} = \frac{(q^4;q^4)^2|\gamma_-(e^{2i\nu_{12}})|^2}{(1-e^{2i\nu_{12}})\Theta_{q^4}(q^4e^{2i\nu_{12}})\Theta_{q^2}(q^2e^{2i\nu_{12}})}\,. \tag{44}$$

Finally, recalling that:

$$\begin{aligned}
\Theta_{q^4}(q^2e^{2i\nu_{12}}) &= \theta_4(e^{i\nu_{12}},q^2) = \frac{\theta_4(q^2)}{\theta_3(q)\theta_4(q)}\,\theta_4(e^{i\nu_{12}/2},q)\theta_3(e^{i\nu_{12}/2},q)\,, \\
\Theta_{q^4}(q^4e^{2i\nu_{12}}) &= \frac{\theta_1(e^{i\nu_{12}},q^2)}{-i\sqrt{q}e^{i\nu_{12}}} = \frac{\theta_4(q^2)}{\theta_3(q)\theta_4(q)}\frac{\theta_1(e^{i\nu_{12}/2},q)\theta_2(e^{i\nu_{12}/2},q)}{-i\sqrt{q}e^{i\nu_{12}}}\,,
\end{aligned} \tag{45}$$

we end up obtaining:

$$\begin{aligned}
&\prod_{\sigma=\pm}\frac{(q^4;q^4,q^4)^2}{(q^2;q^4,q^4)^2}\frac{(q^4e^{2i\sigma\nu_{12}};q^4,q^4)^2}{(q^2e^{2i\sigma\nu_{12}};q^4,q^4)^2} \\
&= \frac{1}{(q^2;q^4)^4}\frac{\sqrt{q}(q^4;q^4)^2|\rho^2\gamma_-(e^{2i\nu_{12}})|^2}{2\sin(\nu_{12})\left(\frac{\theta_4(q^2)}{\theta_3(q)\theta_4(q)}\right)^2\theta_4(e^{i\nu_{12}/2},q)\theta_3(e^{i\nu_{12}/2},q)\theta_1(e^{i\nu_{12}/2},q)\theta_2(e^{i\nu_{12}/2},q)}\,.
\end{aligned} \tag{46}$$

After a major cancellation of terms between numerator and denominator we end up with the following expression:

$$A(\nu_1,\nu_2)=\frac{(q^2;q^2)^4(q;q^2)^4}{(q^2;q^4)^8}\frac{16q\cos^2((p(\nu_1)+p(\nu_2))/2)}{\cosh(\gamma)-\cos(\nu_{12})}\frac{|\rho^2\gamma_-(e^{2i\nu_{12}})|^2}{\frac{\theta_3^2(e^{i\nu_{12}/2},q)}{\theta_3^2(q)}}\,, \tag{47}$$

A similar analysis can be done for the weight $A(\nu_1+\pi,\nu_2)$. To unify both weights we let us introduce the following notation $A_-(\nu_1,\nu_2)=A(\nu_1,\nu_2)$ and $A_+(\nu_1,\nu_2)=A(\nu_1+\pi,\nu_2)$. Finally we have:

$$\begin{aligned}A_\sigma(\nu_1,\nu_2)&=16q\frac{(q^2;q^2)^4(q;q^2)^4}{(q^2;q^4)^8}\frac{|\rho^2\gamma_-(e^{2i\nu_{12}})|^2}{\frac{\theta_3^2(e^{i\nu_{12}/2},q)}{\theta_3^2(q)}}\\&\times\left[\frac{\cos^2((p(\nu_1)+p(\nu_2))/2)}{\cosh(\gamma)-\cos(\nu_{12})}\delta_{\sigma,-}+\frac{\theta_3^2(e^{i\nu_{12}/2},q)}{\theta_4^2(e^{i\nu_{12}/2},q)}\frac{\sin^2((p(\nu_1)+p(\nu_2))/2)}{\cosh(\gamma)+\cos(\nu_{12})}\delta_{\sigma,+}\right].\end{aligned} \tag{48}$$

The final steps express these weights using the $\beta$ parametrization. To do so, we take $q$ to be the elliptic nome $q=e^{-\frac{\pi K'}{K}}$ and $\nu=\frac{\pi\beta}{2K}$. We notice that

$$\rho^2\gamma(\xi_2^2/\xi_1^2)=(q^2;q^4)^2\mathcal{A}_-(\beta_-)\,, \tag{49}$$

where

$$\mathcal{A}_\sigma(\beta_-)\equiv\exp\left[-\sum_{k=1}^{\infty}\frac{\sinh^2[k\epsilon(1-\beta_-/iK')]}{\sinh(2k\epsilon)\cosh(k\epsilon)}\frac{e^{-\sigma k\epsilon}}{k}\right], \tag{50}$$

and $\epsilon\equiv\frac{\pi K'}{K}$. Thus after a fairly lengthy and tedious algebra, we get to:

$$\begin{aligned}A_\sigma(\beta_1,\beta_2)&=4\sqrt{q}kk'\left(\frac{2K}{\pi}\right)^2\frac{\vartheta_A^2(\beta_-)}{\vartheta_d^2(\beta_-,k)}\\&\times\left[\frac{\cos^2((p(\beta_1)+p(\beta_2))/2)}{\cosh\left(\frac{\pi K'}{K}\right)-\cos\left(\frac{\pi\beta_-}{K}\right)}\delta_{\sigma,-}+\frac{\mathrm{dn}^2(\beta_-)}{k'}\frac{\sin^2((p(\beta_1)+p(\beta_2))/2)}{\cosh\left(\frac{\pi K'}{K}\right)+\cos\left(\frac{\pi\beta_-}{K}\right)}\delta_{\sigma,+}\right],\end{aligned} \tag{51}$$

with $\vartheta_A^2(\beta_-)\equiv|\mathcal{A}_-(\beta_-)|^2$. In the last step we have used the following identity

$$16q\frac{(q^2;q^2)^4(q;q^2)^4}{(q^2;q^4)^4}=4\sqrt{q}\,(\theta_2(q)\theta_4(q))^2=4\sqrt{q}kk'\left(\frac{2K}{\pi}\right)^2. \tag{52}$$

The expression (51) correspond to the $B$-weights we were looking for. We can now use them and the two-spinon dispersion relation to integrate over $(\beta_1,\beta_2)$.

### Evaluating the weights $B^{(\sigma)}(\beta_1,\beta_2)$ in terms the 2-spinon energy-momentum dispersion relation

From the expression (19) for LDSF$_{(2)}$, we see that it consists of the sum of the two-spinon continuum weighted by $A^{(+)}(\{\beta\})$ plus the same region shifted by $\pi$ weighted by $A^{-)}(\{\beta\})$. By noticing that a shift in $2K$ in one of the parameters $\beta$ implies a change in the weights $A^{(+)}\leftrightarrow A^{(-)}$, the preceding description is equivalent of weighting the sheets $C_\sigma$ with the weights $A^{(\sigma)}$ for $\sigma=\pm$ and using as the solution to the energy-momentum equations the expressions **without a shift of $2K$.** We can now simply use the Dirac deltas to get rid of the integrals. Let us define:

$$J(\beta_1,\beta_2)=2\left(\frac{2K}{\pi}\right)^2\left|\frac{\partial E}{\partial\beta_1}\frac{\partial P}{\partial\beta_2}-\frac{\partial E}{\partial\beta_2}\frac{\partial P}{\partial\beta_1}\right| \tag{53}$$

Then we can write the expression for $S(Q,\omega)$ as follows

$$S^{zz}_{(2)}(Q,\omega)=\sum_{\sigma\in\pm}\frac{A_\sigma(Q,\omega)}{J_\sigma(Q,\omega)}\mathbb{I}_{(Q,\omega)\in C_\sigma} \tag{54}$$

Now, let us work out a nice and compact expression for $S_2^{zz}(Q,\omega)$. For this we recall the following results [20] that come from solving the two-spinon dispersion relation in terms of $(Q,\omega)$

$$\begin{aligned}
\beta_+^{(\sigma)}(Q,\omega) &= -\frac{1+\kappa}{2} F\left[\arcsin\left(\frac{\omega_0}{\omega}\right), \kappa\right] \\
\beta_-^{(\sigma)}(Q,\omega) &= \mathrm{dn}^{-1}\left(\frac{1+\sigma\cos(Q)}{|\sin(Q)|}\sqrt{\frac{\omega^2-\kappa\omega_0^2+T}{\omega^2+\kappa\omega_0^2-T}}, k\right) \\
\kappa &= \frac{1-k'}{1+k'}, \qquad \omega_0(Q) = \frac{2I}{1+\kappa}\sin(Q), \qquad I = \frac{JK}{\pi}\sinh\left(\frac{\pi K'}{K}\right) \\
T &= T(Q,\omega) = \sqrt{\omega^2-\kappa^2\omega_0^2}\sqrt{\omega^2-\omega_0^2} \\
J_\sigma(Q,\omega) &= 2\left(\frac{2K(\kappa)}{\pi}\right)^2 \frac{\omega T W_\sigma}{\omega_0^2} \\
W_\sigma &= W_\sigma(Q,\omega) = \sqrt{\kappa^2\frac{\omega_0^4}{\omega^4} - \left(\frac{T}{\omega^2}+\sigma\cos(Q)\right)^2}
\end{aligned} \tag{55}$$

This results into the following expression

$$\begin{aligned}
S_{(2)}^{zz}(Q,\omega) &= \sum_{\sigma\in\pm} \frac{A_\sigma(Q,\omega)}{J_\sigma(Q,\omega)} \mathbb{I}_{(Q,\omega)\in C_\sigma} \\
&= 4\sqrt{q}kk'\left(\frac{2K}{\pi}\right)^2 \sum_{\sigma\in\pm} \frac{1}{J_\sigma(Q,\omega)} \frac{|\mathcal{A}_-(\beta_-^{(\sigma)})|^2}{\vartheta_d^2(\beta_-^{(\sigma)},k)} \left[\frac{\sin^2(Q/2)}{\cosh\left(\frac{\pi K'}{K}\right) - \cos\left(\frac{\pi\beta_-^{(\sigma)}}{K}\right)}\delta_{\sigma,-}\right. \\
&\quad \left. + \frac{\mathrm{dn}^2(\beta_-^{(\sigma)})}{k'} \frac{\sin^2(Q/2)}{\cosh\left(\frac{\pi K'}{K}\right) + \cos\left(\frac{\pi\beta_-^{(\sigma)}}{K}\right)}\delta_{\sigma,+}\right] \mathbb{I}_{(Q,\omega)\in C_\sigma}
\end{aligned} \tag{56}$$

Let us look at the weight for $\sigma = +$. One can show that

$$\frac{\mathrm{dn}^2(\beta_-^{(+)})}{k'}\sin^2(Q/2) = \left(\sin(Q/2)\frac{1+\cos(Q)}{|\sin(Q)|}\right)^2 \frac{\omega^2-\kappa\omega_0^2+T}{\omega^2+\kappa\omega_0^2-T} = \frac{1+\cos(Q)}{2}\frac{\omega^2-\kappa\omega_0^2+T}{\omega^2+\kappa\omega_0^2-T} \tag{57}$$

After some tedious steps, this allows to write

$$\begin{aligned}
S_{(2)}(Q,\omega) &= 4\sqrt{q}kk'\left(\frac{2K}{\pi}\right)^2 \sum_{\sigma\in\pm} \frac{1}{J_\sigma(Q,\omega)} \frac{|\mathcal{A}_-(\beta_-^{(\sigma)})|^2}{\vartheta_d^2(\beta_-^{(\sigma)},k)} \frac{1}{2}\left[\frac{1-\cos(Q)}{\cosh\left(\frac{\pi K'}{K}\right) - \cos\left(\frac{\pi\beta_-^{(\sigma)}}{K}\right)}\delta_{\sigma,-}\right. \\
&\quad \left. + [1+\cos(Q)]\frac{\omega^2-\kappa\omega_0^2+T}{\omega^2+\kappa\omega_0^2-T}\frac{1}{k'}\frac{1}{\cosh\left(\frac{\pi K'}{K}\right) + \cos\left(\frac{\pi\beta_-^{(\sigma)}}{K}\right)}\delta_{\sigma,+}\right]\mathbb{I}_{(Q,\omega)\in C_\sigma} \\
&= \sqrt{q}k(1+\kappa)^2\frac{\omega_0^2}{\omega T}\frac{1}{\omega^2+\kappa\omega_0^2-T} \sum_{\sigma\in\pm} \frac{1+\sigma\cos(Q)}{W_\sigma} \frac{|\mathcal{A}_-(\beta_-^{(\sigma)})|^2}{\vartheta_d^2(\beta_-^{(\sigma)})} \left[\frac{\omega^2+\kappa\omega_0^2-T}{\cosh\left(\frac{\pi K'}{K}\right) - \cos\left(\frac{\pi\beta_-^{(\sigma)}}{K}\right)}k'\delta_{\sigma,-}\right. \\
&\quad \left. + \frac{\omega^2-\kappa\omega_0^2+T}{\cosh\left(\frac{\pi K'}{K}\right) + \cos\left(\frac{\pi\beta_-^{(\sigma)}}{K}\right)}\delta_{\sigma,+}\right]\mathbb{I}_{(Q,\omega)\in C_\sigma} \\
&= \sqrt{q}k\frac{\omega^2+\kappa\omega_0^2+T}{\omega^3 T} \sum_{\sigma\in\pm} \frac{1+\sigma\cos(Q)}{W_\sigma} \frac{|\mathcal{A}_-(\beta_-^{(\sigma)})|^2}{\vartheta_d^2(\beta_-^{(\sigma)})} \left[\frac{\omega^2+\kappa\omega_0^2-T}{\cosh\left(\frac{\pi K'}{K}\right) - \cos\left(\frac{\pi\beta_-^{(\sigma)}}{K}\right)}k'\delta_{\sigma,-}\right. \\
&\quad \left. + \frac{\omega^2-\kappa\omega_0^2+T}{\cosh\left(\frac{\pi K'}{K}\right) + \cos\left(\frac{\pi\beta_-^{(\sigma)}}{K}\right)}\delta_{\sigma,+}\right]\mathbb{I}_{(Q,\omega)\in C_\sigma}
\end{aligned} \tag{58}$$

where we have used that

$$K(\kappa) = \frac{K}{1+\kappa}\,, \qquad (\omega^2+\kappa\omega_0^2)^2 - T^2 = (1+\kappa)^2\omega_0^2\omega^2 \tag{59}$$

All in all, we obtain

$$\begin{aligned} S_{(2)}(Q,\omega) = \sqrt{q}k\frac{\omega^2+\kappa\omega_0^2+T}{\omega^3 T}\sum_{\sigma\in\pm}\frac{1+\sigma\cos(Q)}{W_\sigma}\frac{|\mathcal{A}_-(\beta_-^{(\sigma)})|^2}{\vartheta_d^2(\beta_-^{(\sigma)})}\Bigg[\frac{\omega^2+\kappa\omega_0^2-T}{\cosh\left(\frac{\pi K'}{K}\right)-\cos\left(\frac{\pi\beta_-^{(\sigma)}}{K}\right)}\frac{1-\kappa}{1+\kappa}\delta_{\sigma,-} \\ + \frac{\omega^2-\kappa\omega_0^2+T}{\cosh\left(\frac{\pi K'}{K}\right)+\cos\left(\frac{\pi\beta_-^{(\sigma)}}{K}\right)}\delta_{\sigma,+}\Bigg]\mathbb{I}_{(Q,\omega)\in C_\sigma}\,, \end{aligned} \tag{60}$$

which after a bit more rewriting corresponds to the main formula given in the main text.
